# Supplementary material for: Automated Feature-Topic Pairing: Aligning Semantic and Embedding Spaces in Spatial Representation Learning
Source: arXiv:2109.11053 source file (2021-09-22)
Supplement: Supplementary file 1 [file appendix.tex]

\newpage

\begin{center}
\textbf{\fontfamily{ppl} \fontsize{13}{0}\selectfont
Appendix
}%
\bigskip
\end{center}

\noindent \textbf{Reproducing the Algorithm.} To claim AutoFTP clearly, we provide the pseudo-code of the learning process of AutoFTP.
As illustrated in Algorithm \ref{alg:framework},
the framework includes three steps: (i) initializing the parameters of PSO, (ii) optimizing multiple objectives of AutoFTP, (iii) and outputting the final spatial embeddings.
The framework takes topic vectors, POI-POI distance graphs, and POI-POI mobility graphs of spatial entities as input, and final semantically-rich embeddings  as output.

For initializing the parameters of PSO (Line 1-5 in Algorithm \ref{alg:framework}), we first generate $M$ particles as a particle swarm.
Then, we initialize the position (topic mask) and velocity of each particle.
Specifically, we sample $K$ values from the uniform distribution $U(0,1)$ as the position vector, and sample $K$ values from the uniform distribution $U(-1,1)$ as the velocity vector.
Next, we update each particle's best known position (pBest) and the swarm's best known position (gBest) based on each particle's position.

For optimizing multiple objectives of AutoFTP (Line 6-20 in Algorithm \ref{alg:framework}), we first check that if the optimization process achieves the termination conditions.
If best topic mask is not found or the training iteration does not surpass the max iteration limitation, 
we optimize the objectives continually.
Otherwise, we output the final spatial representations.
During the optimization process, for one iteration, we utilize one particle to do feature-topic pairing.
Specifically, we first update the velocity of the particle based on the old velocity, the gap between the current position and pBest, and the gap between the current position and gBest. 
Then, we generate a new position vector (topic mask) based on the velocity vector (Line 10-11 in Algorithm \ref{alg:framework}). 
In the two lines, $\omega, \phi_p, \phi_g$ are weights, and $\gamma$ is the learning rate of the corresponding items.
Then, we filter $K$ topics by the topic mask and generate the basic embedding of a spatial entity.
In addition, we align the semantics of the $K$ topics and the features of the basic embedding, and accomplish a downstream task simultaneously (Line 12-15 in Algorithm \ref{alg:framework}).
Moreover, we evaluate the performance of the particle, and update the value of pBest and gBest for next optimization iteration (Line 16-20, in Algorithm \ref{alg:framework}).

For outputting final spatial embeddings (Line 21-23 in Algorithm \ref{alg:framework}), we copy the learned spatial representation as the final semantically-rich representations of spatial entities.

\begin{algorithm}[b] 
  \SetKwInOut{Input}{Input}\SetKwInOut{Output}{Output}
  \Input{
  Topic vectors $[\mathbf{t}_1,\mathbf{t}_2, \cdots, \mathbf{t}_N]$;\newline
  POI-POI distance graphs $[G_1^d,G_2^d,\cdots,G_N^d]$;\newline
  POI-POI mobility graphs $[G_1^m,G_2^m,\cdots,G_N^m]$;\newline
}
\Output{Semantically-rich embeddings $[\mathbf{\tilde{r}}_1,\mathbf{\tilde{r}}_2,\cdots,\mathbf{\tilde{r}}_n]$.
  }
  \tcp{Initializing the parameters of PSO} 
  \For{each particle $i=1,\cdots,M$}{
%   \tcp{$x_i \in \mathbb{R}^{K}$, $U$ is a uniform distribution}
  $x_i \sim U(0,1)$;
    % \tcp{$v_i \in \mathbb{R}^{K}$, $U$ is a uniform distribution }
  $v_i \sim U(-1,1)$;
%   \tcp{Initialize the  partial best position $pBest_i$}
  $pBest_i \leftarrow x_i$;\\
%   \tcp{Initialize the global best position $gBest$ }
  \If{Fitness($gBest$) $>$ Fitness($pBest_i$)}{$gBest \leftarrow pBest_i$;\\}
  }
  \tcp{Optimizing multiple objectives of AutoFTP}
  \While{(Fitness(gBest) $> \epsilon$) and (Iteration $<$ maxIter)}
  {
  \For{each entity $n=1,\cdots,N$}{
  \For{each particle $i=1,\cdots,M$}{
  \For{each dimension $k=1,\cdots,K$}{
%   \tcp{$\omega, \phi_p, \phi_g$ are weights of each item.}
   $v_{i,d} \leftarrow \omega \cdot v_{i,d} + \phi_p \cdot (pBest_{i,d}-x_{i,d}) + \phi_g \cdot (gBest_{d}-x_{i,d})$;\\
  }
%   \tcp{$\gamma$ is the learning rate.}
  $x_i \leftarrow x_i + \gamma v_i$;\\
%   \tcp{Filter k topics from all topics.}
  $\mathbf{\check{t}}_n \leftarrow \mathbf{t}_n \oplus x_i$;\\
%   \tcp{Obtain the basic embedding}
%   $\mathbf{r}^n = Mean(\mathcal{L}_R^d(GCN(G_n^d)) , \mathcal{L}_R^m(GCN(G_n^m)))$;\\
    $\mathbf{r}^n = GCN(G_n^d,G_n^m)$;\\
    Calculate the value of $\mathcal{L}_R,\mathcal{L}_P,\mathcal{L}_C, \mathcal{L}_{Reg}$.\\
%   $l_R = Mean(\mathcal{L}_R^d, \mathcal{L}_R^m)$;\\
% %   \tcp{Semantic Alignment}
%   $l_P = \mathcal{L}_P(\mathbf{\check{t}}^n,\mathbf{r}^n)$;
%   $l_C = \mathcal{L}_C(\mathbf{S},\mathbf{S}')$;\\
% %   \tcp{Downstream Regression Task}
%   $l_{Reg} = \mathcal{L}_{Reg}(\mathbf{r}_n)$;\\
%   \tcp{Calculate Fitness value}
%   $Fitness(x_i) = \mathcal{L}_R + \mathcal{L}_P + \mathcal{L}_C + \mathcal{L}_{Reg}$;\\
%   \tcp{Update the value of $pBest_i$ and $gBest$}
  \If{Fitness($pBest_i$) $>$ Fitness($x_i$)}{
  $pBest_i \leftarrow x_i$;\\
  \If{Fitness($gBest$) $>$ Fitness($pBest_i$)}{
  $gBest \leftarrow pBest_i$;\\
  }
  }
  }
  }
  Iteration++;\\
  }
  \tcp{Outputting final spatial embeddings}
  \For{each entity $n=1,\cdots,N$}{
  $\mathbf{\tilde{r}}_n \leftarrow \mathbf{r}_n$
  }
  \caption{ Automatic Feature-Topic Pairing (AutoFTP).}
  \label{alg:framework}
%   \vspace{0.3cm}
\end{algorithm}
